# Supplementary material for: Three dimensions, two microscopes, one code: automatic differentiation for x-ray nanotomography beyond the depth of focus limit
Source: arXiv:1905.10433 source file (2019-05-24)
Supplement: Supplementary file 1 [file sciadv_supp_v1.pdf]

# Supplementary material on “Three dimensions, two microscopes, one code…”

This supplement adds additional information to the above paper in connection with the mathematical notation of the forward model (Sec. 1), and computational experiments on a protein molecule as a second test specimen (Sec. 1.1).

## 1 Linear algebraic notation of the forward model

We start with the incident wave $\boldsymbol{\psi}_0$ which is an $M \times 1$ column vector, where $M$ is total number of pixels of the detector. For viewing direction $\theta$, the object function $\boldsymbol{x}$, which is an $N \times 1$ column vector with $N$ being the total number of object voxels, has to be rotated with the rotation operator $\boldsymbol{R}_\theta$. The product $\boldsymbol{R}_\theta \boldsymbol{x}$ is another $N \times 1$ column vector representing the rotated object.

For the modulation on the wavefront by the first object slice, we use a sampler matrix $\boldsymbol{S}_{j,p}$ to extract that slice from $\boldsymbol{x}$ as a sparse column vector. $\boldsymbol{S}_{j,p}$ is an $M \times N$ matrix that can be written a concatenation of a zero matrix, an identity matrix, and another zero matrix:

$$\boldsymbol{S}_{j,p} = [\text{zeros}(M, P), \mathbb{1}, \text{zeros}(M, N - P - M)]. \tag{1}$$

A visual representation of $\boldsymbol{S}_{j,p}$ is the following as follows:

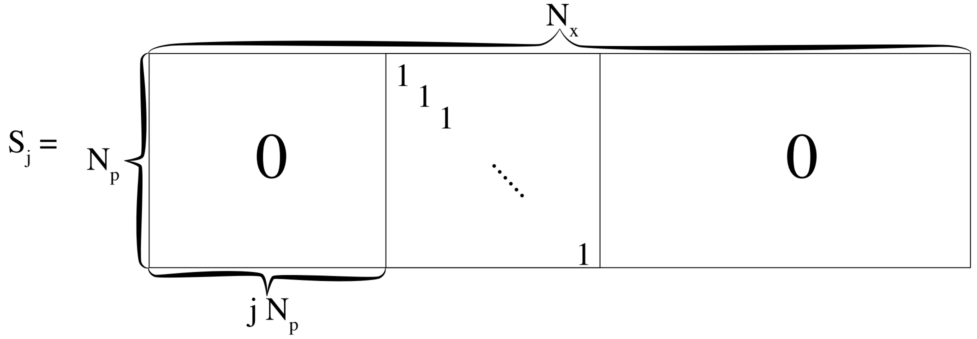

The product $\boldsymbol{S}_{j,p}\boldsymbol{R}_\theta\boldsymbol{x}$ is then an $M \times 1$ column vector in the form of

$$\boldsymbol{S}_{j,p}\boldsymbol{R}_\theta\boldsymbol{x} = \begin{bmatrix} x_{j,0} \\ x_{j,1} \\ \vdots \\ x_{j,M-1} \end{bmatrix} \tag{2}$$

The modulation is in fact the element-wise product between $\boldsymbol{S}_{j,p}\boldsymbol{R}_\theta\boldsymbol{x}$ and $\boldsymbol{\psi}_0$, which should be written as

$$\boldsymbol{\psi}_0' = \text{diag}(\boldsymbol{S}_{j,p}\boldsymbol{R}_\theta\boldsymbol{x})\boldsymbol{\psi}_0. \tag{3}$$

Again, the resulting $\boldsymbol{\psi}_0'$ should be a $M \times 1$ column vector. To propagate the wavefront to the next slice, we define propagation operator $\boldsymbol{P}_{\Delta z}$. The product $\boldsymbol{P}_{\Delta z}\boldsymbol{\psi}_0'$ should be equivalent to the convolution $\phi_0'(x,y) * h(x,y)$. The matrix form of $\boldsymbol{P}_{\Delta z}$ should then be

$$\boldsymbol{P}_{\Delta z} = \begin{bmatrix} \text{flatten}[h(x,y)] \\ \text{flatten}[h(x+1,y)] \\ \vdots \\ \text{flatten}[h(x,y+1)] \\ \text{flatten}[h(x+1,y+1)] \\ \vdots \\ \text{flatten}[h(x+L-1,y+L-1)] \end{bmatrix} \tag{4}$$

where $L$ is the side length of the wavefront array; in the case of a square array, we have $M = L \times L$. Then,

$$\begin{aligned} \boldsymbol{\psi}_1 &= \boldsymbol{P}_{\Delta z}\boldsymbol{\psi}_0' \\ &= \boldsymbol{P}_{\Delta z}\text{diag}(\boldsymbol{S}_{j,p}\boldsymbol{R}_\theta\boldsymbol{x})\boldsymbol{\psi}_0. \end{aligned} \tag{5}$$

The above operations are repeated for all the $J$ slices, so the exiting wave should be

$$\begin{aligned} \boldsymbol{\psi}_J &= \boldsymbol{M}_{\boldsymbol{x},\theta,s}\boldsymbol{\psi}_0 \\ &= \prod_j^J [\boldsymbol{P}_{\Delta z}\text{diag}(\boldsymbol{S}_{j,p}\boldsymbol{R}_\theta\boldsymbol{x})]\boldsymbol{\psi}_0. \end{aligned} \tag{6}$$

Finally, the wavefront at the detector plane is reached by doing free space propagation:

$$\boldsymbol{\psi}_d = \boldsymbol{P}_{z_f}\boldsymbol{\psi}_J. \tag{7}$$

This leads to the detectable signal $I_d = \boldsymbol{\psi}_d^\dagger\boldsymbol{\psi}_d$ where $\dagger$ is the complex conjugate.

## 1.1 Studies on a protein sample

In order to further explore the properties of our reconstruction method, we carried out computational experiments on a second, soft matter object: the 3D structure of the surface adhesin complex from *Mycoplasma genitalium* known as NAP. This structure was determined by electron microscopy (*1*), and was retrieved as ID EMD-3756 from the *EMDataBank* (*2*). We mapped the 3D electron density onto a $(256)^3$ voxel grid with 0.67 nm voxel size, assuming that the normalized electron density represented a volume filling fraction for protein. We then used the stoichiometric average of all 20 amino acids as a stand-in for a generic protein (*3*) with a maximum density of 1.35 g/cm$^3$, with 5 keV x-ray refractive index paraemters of $\delta = 1.0 \times 10^{-7}$ and $\beta = 8.5 \times 10^{-10}$ based on tabulated data (*4*). Full-field propagation phase contrast data were generated using the forward model described in Eq. 6 for 500 orientation angles between 0° and 360°; one such projection image is shown as an inset in Fig. 1(a). For ptychography, we used a Gaussian probe with $\sigma_x = \sigma_y = 6.7$ nm and a maximum phase of 0.5 to generate $23 \times 23 = 529$ diffraction patterns for each of the 500 sample orientations between 0 and 360°. These procedures for generating simulated data were identical to those used for the silicon cone-shaped object described in the main manuscript.

The full-field tomography reconstruction was reconstructed on a workstation with with two Intel Xeon E5-2620v4 CPUs, two NVIDIA Quadro P4000 GPUs (8 GB GPU memory each), and 512 GB RAM. Due to the higher requirement on memory and processor multithreading capability, the ptychography reconstruction on the protein sample was performed on the computing cluster Cooley at the Argonne Leadership Computing Facility. Each of the 128 nodes of this cluster is equipped with two 2.4 GHz Intel Haswell E5-2620 v3 CPUs (12 cores total) and 384 GB RAM. For both modes, reconstruction of the dataset was done using $\alpha_d = 1 \times 10^{-9}$ and $\alpha_b = 1 \times 10^{-10}$. In this case we used $\gamma = 0$ to exclude the total variation (TV) term in the cost function, as its anisotropic smoothing effect (along each axis) was a more match to the isotropically smooth character of the object. The full-field reconstruction voxel grid was initialized using $\delta = 8 \times 10^{-7}$ and $\beta = 8 \times 10^{-8}$, which is slightly lower than the phase shifting value for voxels with full protein density. We used a minibatch size of 10 for full-field, and 1 for ptychography, and set the iterator to stop automatically once the decrement of the total loss was less than $3\%$. Using GPU acceleration provided by TensorFlow, the computation for full-field imaging converged after 5 epochs, or 538 s. The ptychography reconstruction of this sample on the computing cluster Cooley consumed a total of 350 core hours.

Figure 1(a) shows the two $xz$-cross sections of the $\delta$-map of the ground truth object. The positions of these cross sections are marked by the yellow dashed lines in $xy$-cross section in the third column. The "halo" around the molecule comes from the original electron tomography data;

it provides a way to examine the ability of our algorithm in providing a faithful reconstruction. The results obtained from full-field imaging are shown in Fig. 1(b). Under the joint effect of finite support constraint and sparsity constraint, the halo around the protein is not well represented, but the core molecular structure is faithfully reconstructed. We note here that the removal of the halo is not a direct consequence of shrink-wrap. Even if a rough, cylindrical finite support mask is used without shrinkwrap, the output image is still free of halos. This can be an advantageous feature if one desires to eliminate such halos, which can be a problem in electron microscopy and phase contrast microscopy (*5*). However, when one wants to preserve weak and diffusive features in the sample, the loss of low contrast features on the object's periphery will become undesirable. The situation is improved in the ptychographic reconstructions shown in Fig. 1(c); here we see that the diffusive halo is reconstructed faithfully, along with the core molecular structure.

The difference between the full-field and the ptychography reconstruction results can be viewed more quantitatively in Fig. 2, where a line profile crossing the center of a four-fold symmetric motif is shown for the true object, the full-field reconstruction, and the ptychography reconstruction. Both the true object and the ptychography reconstruction show side lobes corresponding to the halo, while the full-field result does not. Even in the molecule's center, the ptychography reconstruction is quantitatively closer to the ground truth than the full-field result.

In contrast to our multislice full-field and ptychography results, the result of the pure-projection approximation (ER+FBP) reconstruction shown in the last row of Fig. 1 contains a large amount of artifacts and loss of structural information, although it indeed converged at a solution that partially resolves the major motifs of the macromolecule. In ER phase retrieval, we assumed that the 2D object function at each projection angle lies in the middle of the actual object. Since this does not properly account for the depth information of features, the presence of artifacts is as expected.

One last point to note is that for both full-field and ptychography modes, the reconstructed maps of $\beta$, the absorptive part of the x-ray refractive index, were of low quality (images not shown here). This is of course explained by the weak contrast provided by x-ray absorption for a biological specimen at 5 keV photon energy.

# References


1. M. P. Scheffer, *et al.*, *Molecular Microbiology* **105**, 869 (2017).

2. C. L. Lawson, *et al.*, *Nucleic Acids Research* **44**, D396 (2016).

3. R. A. London, M. D. Rosen, J. E. Trebes, *Applied Optics* **28**, 3397 (1989).

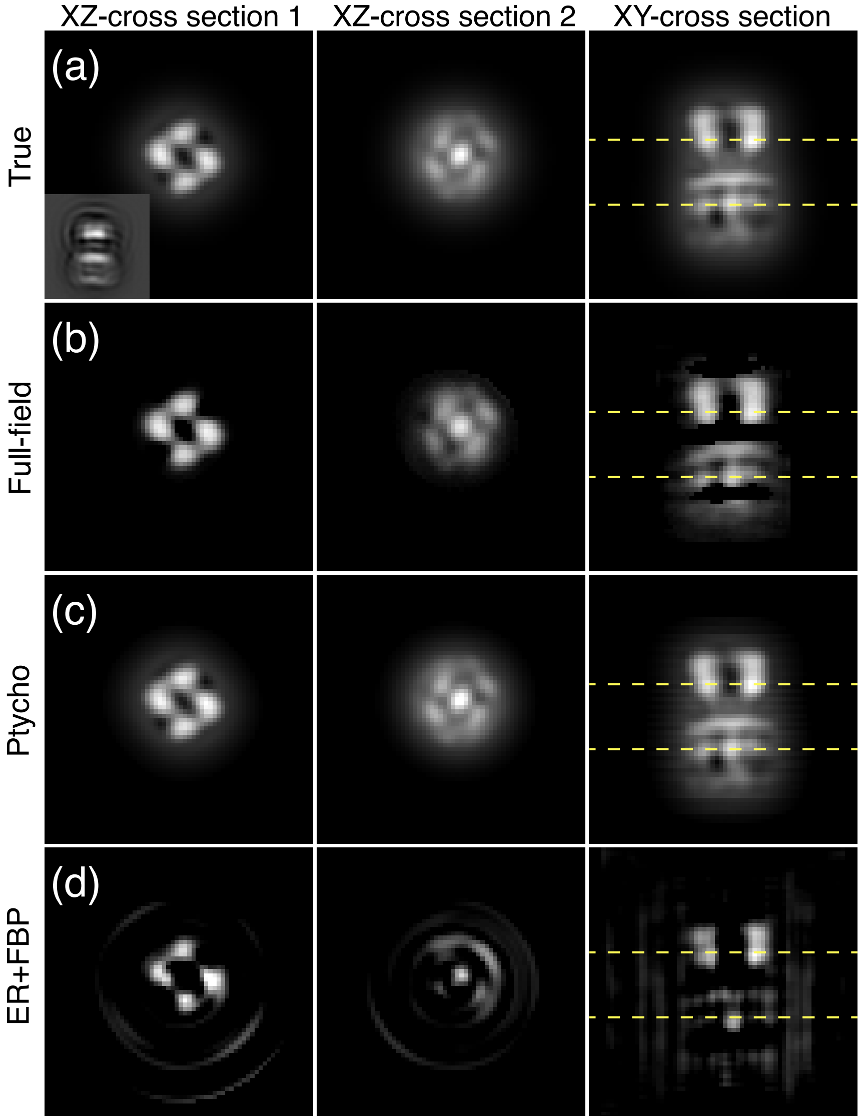


Figure 1: The NAP protein object sectioned from the two $xz$-planes (column 1 and 2) marked by the yellow dashed lines in the $xy$-cross section (column 3). Images of the phase shifting part of the x-ray refractive index $\delta$ presented here are from (a) the true object, (b) the object reconstructed using 360°-full-field data, (c) the object reconstructed using 360°-ptychography data, and (d) the object reconstructed using a conventional pure-projection approximation tomography approach (denoted here by ER+FBP).

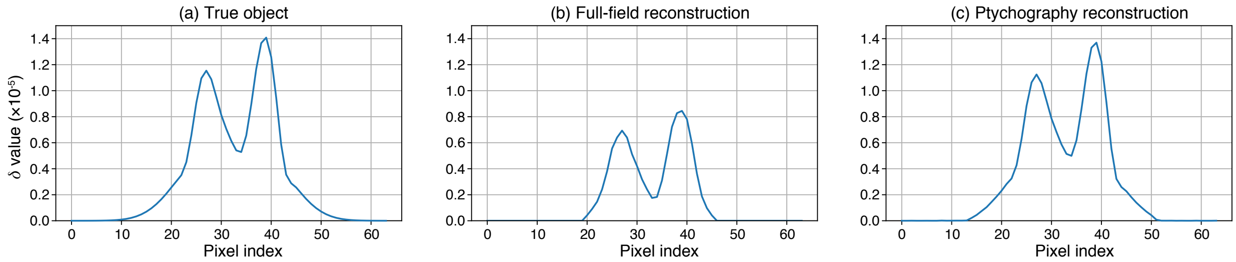


Figure 2: Line profiles across the phase-shifting part of the refractive index $\delta$ for the NAP protein sample. The plots are respectively for (a) the true object, (b) the full-field reconstruction, and (c) the ptychography reconstruction. The locations of the line profile are indicated by the upper dashed line in the third column of Fig. 1. The physical pixel size is 0.67 nm.

4. B. L. Henke, E. M. Gullikson, J. C. Davis, *Atomic Data and Nuclear Data Tables* **54**, 181 (1993).

5. M. E. Kandel, M. Fanous, C. Best-Popescu, G. Popescu, *Biomedical Optics Express* **9**, 623 (2018).
